# Supplementary material for: UGC-VideoCaptioner: An Omni UGC Video Detail Caption Model and New Benchmarks
Source: arXiv:2507.11336 source file (2025-10-05)
Supplement: Supplementary file 1 [file appendix.tex]

\section{Evaluation on UGC-VideoCap}

\section{UGC-VideoCaptioner Training Detail}
We used a two-stage training, which included full modal distillation sft and secondary refinement GRPO training. All experiments were trained at 8xH200, and details of the training parameters are referenced in Tables~\ref{grpo} and~\ref{}.

\begin{table}[h]
\centering
\caption{Key Configuration Parameters for GRPO Training}
\begin{tabular}{ll}
\hline
\textbf{Parameter} & \textbf{Value} \\
\hline
Model & Qwen2.5-Omni-3B \\
Frames & 32 \\
Training Type & LoRA \\
LoRA Rank & 16 \\
LoRA Alpha & 32 \\
Target Modules & all-linear \\
Torch Dtype & bfloat16 \\
Max Completion Length & 1024 \\
Max Input Length & 8192 \\
Number of Epochs & 1 \\
Train Batch Size & 2 \\
Eval Batch Size & 2 \\
Learning Rate & 1e-5 \\
Gradient Accumulation Steps & 1 \\
Warmup Ratio & 0.05 \\
Deepspeed Config & zero2 \\
Number of Generations & 8 \\
Temperature & 1.0 \\
Top-p & 0.99 \\
Top-k & 50 \\
\hline
\end{tabular}
\label{grpo}
\end{table}
